# Supplementary material for: Blind Super-Resolution Kernel Estimation using an Internal-GAN
Source: arXiv:1909.06581 source file (2020-01-07)
Supplement: Supplementary file 1 [file appendix.tex]

\section*{Appendix-- Deriving the SR-kernel for SR$\times$4  from  the SR-kernel for SR$\times$2}
\label{appendix}
This can be shown in 1D, by analyzing the result of convolving some kernel $k$ with any subsampled signal $x$. We show that it is equivalent to first convolving with $k_{sparse}$ and then subsampling.
\[ \label{eq1}
\begin{split}
  \left\{\vphantom{\left(\sum_{1}^2\right)}k \:\boldsymbol{*}\: x[2 \: \boldsymbol{\cdot}\:]\right\}[n] &= 
  \sum_{l=-\infty}^{\infty}\left(\vphantom{\sum_{1}^2}k[n-l]\cdot x[2l]\right)\\
  \intertext{We can substitute $m:=2l$ and use Kronecker Delta Comb to enforce $m$ to be even;}
  &= \sum_{l=-\infty}^{\infty}\left(\left(\sum_{m=-\infty}^{\infty}\delta[m-2l]\right) \cdot k[n-\frac{m}{2}] \cdot  x[m]\right)\\
    \intertext{Assuming both signals are of finite energy, changing the summation order is allowed. Adding $2n$ does not change the result of the Kronecker Delta Comb;}
    &= \sum_{m=-\infty}^{\infty}\left(\left(\sum_{l=-\infty}^{\infty}\delta[2l+2n-m] \cdot k\left[\frac{1}{2}(2n-m)\right]\right) \cdot  x[m]\right)\\
    \intertext{This formulates a convolution;}
    &= \left\{ \left(\sum_{l=-\infty}^{\infty}\delta[\:\boldsymbol{\cdot}\:-2l] \cdot k\left[\frac{\:\boldsymbol{\cdot}\:}{2}\right] \right) \:\boldsymbol{*}\: x\right\} [2n]\\
    \intertext{The Kronecker Delta Comb zeroizes for odd inputs, we therefore obtain $k_{sparse}$;}
    &=\left\{\vphantom{\left(\sum_{1}^2\right)}k_{sparse} \:\boldsymbol{*}\: x\right\}[2n]
\end{split}
\]
